# Supplementary material for: Causal survival embeddings: non-parametric counterfactual inference under censoring
Source: arXiv:2306.11704 source file (2023-06-20)
Supplement: Supplementary file 1 [file Appendix1.tex]

\chapter{Complementary information}
\label{app:complement}

Additional material. For example long mathematical derivations could be
given in the appendix. Or you could include part of your code that is
needed in printed form. You can add several Appendices to your thesis (as
you can include several chapters in the main part of your work).

\section{Including \Rp code with verbatim}
A simple (rather too simple, see~\ref{App:listings}) way to include code or
{\it R} output is to use 
\texttt{verbatim}. It just prints the text however it is (including all
spaces, ``strange'' symbols,...) in a slightly different font.
\begin{verbatim}
## loading packages
library(RBGL)
library(Rgraphviz)
library(boot)

## global variables
X_MAX <- 150

   This allows me to put as many s  p a   c es   as I want.
I can also use \ and ` and & and all the rest that is usually only 
accepted in the math mode.

I can also make as 
                  many 
             line 
    breaks as 
I want... and
             where I want. 
\end{verbatim}

But really recommended,  much better is the following:

\section{Including \Rp code with the \emph{listings} package}\label{App:listings}
However, it is much nicer to use the \emph{listings} package to include \Rp
code in your report. It allows you to number the lines, color the comments
differently than the code, and so on.
All the following is produced by simply writing
\verb! \lstinputlisting{Pictures/picture.R} !  in your \LaTeX\ ``code'':

\lstinputlisting{Pictures/picture.R}

or \verb!\lstinputlisting{/u/maechler/R/Pkgs/sfsmisc/R/ellipse.R}! :

%\lstinputlisting{../RCode/ellipse.R}% was /u/maechler/R/Pkgs/sfsmisc/R/ellipse.R

\section{Using \texttt{Sweave} (or \texttt{knitr}) to include \Rp code (and more) in your report}
The easiest (and most elegant) way to include \Rp code and its output (and
have all your figures up to date with your report) is to use Sweave---or the
\href{https://cran.R-project.org/package=knitr}{\texttt{knitr}} R package with even more possibilities.
% You can find an introduction Sweave in \texttt{/u/sfs/StatSoftDoc/Sweave/Sweave-tutorial.pdf}.

Search the web to find lots of intro material on how to use Sweave or
\href{https://en.wikipedia.org/wiki/Knitr}{knitr (on Wikipedia)}.

%%% Local Variables: 
%%% mode: latex
%%% TeX-master: "MasterThesisSfS"
%%% End: 
