# Supplementary material for: Causal survival embeddings: non-parametric counterfactual inference under censoring
Source: arXiv:2306.11704 source file (2023-06-20)
Supplement: Supplementary file 2 [file Appendix_more_R.tex]

\chapter{2nd Appendix: More sophisticated R code listing} \label{appendix-more-R}

Chapter-wise listing of parts of R code, using
\begin{itemize}
\item \texttt{firstline=n1}
\item \texttt{lastline=n2}
\item \texttt{title=<text>}
\end{itemize}
e.g., for the first example below
\begin{verbatim}
\lstinputlisting[firstline=1,lastline=32,
                 title= \texttt{read\_irwls\_fn.R}]{../RCode/read_irwls_fn.R}
\end{verbatim}

% \section{Chapter 2} \label{app 2}

% \lstinputlisting[firstline=1,lastline=77,
% title=\texttt{analytic\_efficiency.R}]{../RCode/analytic_efficiency.R}
% %\lstinputlisting[firstline=,lastline=]{../RCode/???.R}

\bigskip% or even  \clearpage

%-----------------------------------------------------------------------------------------
\section{Chapter 5} \label{app 5}

% \lstinputlisting[firstline=1,lastline=71,
%                  title=\texttt{loss-fn\_rotated.R}]{../RCode/loss-fn_rotated.R}
\lstinputlisting[firstline=1,lastline=32,
                 title= \texttt{read\_irwls\_fn.R}]{../RCode/read_irwls_fn.R}

\medskip
                 
\lstinputlisting[firstline=1,lastline=45,
                 title=\texttt{plot.psi.R}]{../RCode/plot.psi.R}
%\lstinputlisting[firstline=,lastline=]{../RCode/???.R}
%\lstinputlisting[firstline=,lastline=]{../RCode/???.R}

% \clearpage
%-----------------------------------------------------------------------------------------
% \section{Chapter 7} \label{app 7}

% \lstinputlisting[firstline=1,lastline=35,
%                  title= \texttt{stat.test} from \texttt{lmrob2-fn.R}]{../RCode/lmrob2-fn.R}
% \lstinputlisting[firstline=41,lastline=194,
%                  title=\texttt{M.optimal.ms} from \texttt{lmrob2-fn.R}]{../RCode/lmrob2-fn.R}
%\lstinputlisting[firstline=,lastline=]{../RCode/???.R}
%-----------------------------------------------------------------------------------------

%%% Local Variables:
%%% mode: latex
%%% TeX-master: "MasterThesisSfS"
%%% End:
