# Supplementary material for: Causal survival embeddings: non-parametric counterfactual inference under censoring
Source: arXiv:2306.11704 source file (2023-06-20)
Supplement: Supplementary file 3 [file Appendix2.tex]

\chapter{Yet another appendix....}

\section{Description}
\begin{description}
\item[Something] details.
\item[Something else] other definition.
\end{description}

\section{Tables}
Refer to Table~\ref{tab:example} to see a left justified table with caption
on top.

\begin{table}[ht]
\centering
\caption[Test results]{\label{tab:example}Results.}
\begin{tabular}{ll}
\hline
\textbf{Student} & \textbf{Grade}\\
\hline
Marie  & $6$\\
Alain  & $5.5$\\
Josette  & $4.5$\\
Pierre  & $5$\\
\hline
\end{tabular}
\end{table}

%%% Local Variables: 
%%% mode: latex
%%% TeX-master: "MasterThesisSfS"
%%% End: 
